# Supplementary material for: SummaReranker: A Multi-Task Mixture-of-Experts Re-ranking Framework for Abstractive Summarization
Source: arXiv:2203.06569 source file (2023-05-26)
Supplement: Supplementary file 1 [file appendix_j_old.tex]

% \begin{figure}[h]
%   \centering
%     \includegraphics[width=0.95\columnwidth]{Images/abstractiveness_xsum.png}
%     \caption{\textbf{Novel $n$-grams} with a base PEGASUS model on \textbf{XSum}.}
%     \label{fig:7}
% \end{figure}

% Per \Cref{fig:7}, SummaReranker summaries are slightly more abstractive in terms of 2-grams, 3-grams and 4-grams for diverse beam search on XSum. There is no abstractiveness gain for beam search candidates.


% \begin{figure}[h]
%     \includegraphics[width=0.95\columnwidth]{Images/abstractiveness_reddit.png}
%     \caption{\small \textbf{Novel $n$-grams} with a base PEGASUS model on \textbf{Reddit TIFU}.}
%     \label{fig:8}
% \end{figure}

% We note in \Cref{fig:8} that on Reddit TIFU, SummaReranker candidates are systematically more abstractive in terms of 2-grams, 3-grams and 4-grams. 
